# Supplementary material for: Beyond the False Trade-off: Adaptive EWC for Stealthy and Generalizable T2I Backdoors
Source: arXiv:2605.08280 source file (2026-05-08)
Supplement: Supplementary file 1 [file 6_appendix.tex]

\appendix
\FloatBarrier  % ensure no earlier floats move above the appendix heading

\section{Additional Experimental Details}
\label{app:details}

\subsection{Compute, budgets, and protocol}
\label{app:compute}
All experiments are executed under identical budget policies (number of steps, optimizer, batch scheduling) and start from the same teacher snapshot. Each run initializes a fresh student and uses the exact same random seed set per experiment type. We cache the Fisher statistics once and reuse them across all EWC variants to avoid confounding effects from re-estimation.

\paragraph{Hardware.}
Report the exact GPU model(s) and VRAM (e.g., \emph{1$\times$ NVIDIA A100 80GB}), number of GPUs per run, CPU model, and framework versions (CUDA, PyTorch, diffusers). Also report typical wall-clock time per run and total number of runs.

\paragraph{Reproducibility protocol.}
We fix the data loaders, prompt shuffling, and tokenization versions; we log configuration files and random seeds for each run. Inference cost is unchanged across methods because the regulator and consolidation operate only during training.

\subsection{Hyperparameters and schedules}
\label{app:hparams}
We provide the full grid and the selected settings per trigger family. The regulator parameters $(\alpha,\beta,\lambda_{\min},\lambda_{\max})$ are shared unless stated otherwise. The Fisher surrogate uses a clean prompt subsample of size $N$ (disjoint from all evaluations).

% --- table pinned "here" to avoid jumping above headings ---
\begin{table}[H]
\centering
\caption{Full hyperparameter specification per trigger family (reproduces Sec.~\ref{sec:experiments}).}
\label{tab:app_hparams}
\setlength{\tabcolsep}{3pt}
\footnotesize
\resizebox{\columnwidth}{!}{%
\begin{tabular}{lcccccccc}
\toprule
Trig. & lr & steps & $w_b$ & $w_u$ & $w_x$ & $\lambda_0$ & $\alpha$ & $\lambda$-range \\
\midrule
Syntactic & $4.5{\times}10^{-6}$ & 1350 & 1.65 & 1.15 & 0.08 & 0.09 & 0.85 & [0.05, 0.50] \\
Unicode   & $4.5{\times}10^{-6}$ & 1350 & 1.65 & 1.15 & 0.08 & 0.09 & 0.85 & [0.05, 0.50] \\
Phrase    & $1.5{\times}10^{-5}$ &  220 & 1.30 & 1.00 & 0.05 & 0.09 & 0.70 & [0.05, 0.50] \\
\bottomrule
\end{tabular}%
}
\end{table}

\subsection{Fisher subsampling and prompt pool}
\label{app:fisher_pool}
We estimate a diagonal Fisher at $\theta{=}\theta^\ast$ via squared gradients of a clean cosine surrogate, averaged over $N{=}512$ clean prompts unless noted. The surrogate is
\[
\mathcal{L}_{\text{sur}}(c;\theta) = 1 - \cos\!\big(S_\theta(c),\,T(c)\big),
\]
with gradients taken at $\theta{=}\theta^\ast$. The clean prompt pool used for Fisher estimation is disjoint from all evaluation prompts and is held fixed across methods to ensure comparability.
